# Supplementary material for: Informational Memory Shapes Collective Behavior in Intelligent Swarms
Source: arXiv:2409.06660 source file (2025-12-16)
Supplement: Supplementary file 1 [file Spinner_supp.pdf]

# Supplementary Material

## CONTENTS

|                                                                                       |    |
|---------------------------------------------------------------------------------------|----|
| I. Model                                                                              | 1  |
| A. Spontaneous symmetry breaking                                                      | 1  |
| 1. Population dynamics in memory space                                                | 1  |
| 2. Fix points and steady states                                                       | 2  |
| 3. Effective potential landscape and quadratic approximation                          | 3  |
| B. Population distribution of $N_+$ for $M = 1$ and the symmetry for transient memory | 5  |
| C. Curmudgeons bias the double-well                                                   | 6  |
| D. A contrarian oscillates the demographics                                           | 6  |
| II. Supplementary experiment trajectories                                             | 8  |
| III. Algorithms for robotic agents                                                    | 10 |
| IV. Simulation                                                                        | 11 |
| A. Molecular dynamics simulation                                                      | 11 |
| B. Simplified state simulation                                                        | 11 |
| V. Supplementary movies                                                               | 12 |
| References                                                                            | 12 |

## I. MODEL

### A. Spontaneous symmetry breaking

#### 1. Population dynamics in memory space

We describe the evolution of the probability  $n_+$  that an agent is in the  $+$  state, and for the memory state  $s_m$ , ( $m = 0, \dots, M$ ).

If we define  $\tau_c^{-1}$  the collision rate, we have

$$s_m(t + \Delta t) = s_m(t) \left( 1 - \frac{\Delta t}{\tau_c} \left( 1 - \frac{M-m}{M} p_- - \frac{m}{M} p_+ \right) \right) + \frac{\Delta t}{\tau_c} \left( s_{m+1} \frac{m+1}{M} p_- + s_{m-1} \frac{M-m+1}{M} p_+ \right). \quad (\text{S1})$$

Here

$$p_+ \equiv n_+(1 - \eta) + (1 - n_+)\eta, \quad p_- = 1 - p_+ \quad (\text{S2})$$

where  $\eta$  is the probability of measuring the wrong state. In fact there are two ways a collision can result in measuring an agent in the state  $+$ : either we interact with an agent in the state  $-$  and measure the correct state  $n_+(1 - \eta)$  or we interact with an agent in the state  $-$  and measure the wrong state  $(1 - n_+)\eta$ .

Therefore the time evolution of the memory state probability  $s_n(t)$  is given by

$$\frac{ds_m(t)}{dt} = T_{mm'}(n_+(t))s_{m'}(t) \quad (\text{S3})$$

where the matrix  $T_{mm'}$  is given by Eq.S1. For example, for  $M = 5$  the matrix  $T(n_+)$  is

$$\begin{pmatrix} p_- - 1 & \frac{p_-}{5} & 0 & 0 & 0 & 0 \\ p_+ & \frac{p_+}{5} + \frac{4p_-}{5} - 1 & \frac{2p_-}{5} & 0 & 0 & 0 \\ 0 & \frac{4p_+}{5} & \frac{2p_+}{5} + \frac{3p_-}{5} - 1 & 0 & 0 & 0 \\ 0 & 0 & \frac{3p_+}{5} & \frac{3p_+}{5} + \frac{2p_-}{5} - 1 & \frac{4p_-}{5} & 0 \\ 0 & 0 & 0 & \frac{2p_+}{5} & \frac{4p_+}{5} + \frac{p_-}{5} - 1 & p_- \\ 0 & 0 & 0 & 0 & \frac{p_+}{5} & p_+ - 1 \end{pmatrix} \quad (\text{S4})$$

At this point we can assume that the state of each agent, + or -, is determined by its internal memory state. In this case, the probability  $n_+$  of being in the state + is given by

$$n_+(t) = \sum_{m=\frac{M+3}{2}} s_m(t). \quad (\text{S5})$$

We can relax this assumption and assume that, instead of aligning instantly their state with their memory state, the agents update their state with rate  $\tau_u$ , essentially the collision rate of the physical agents. In this case we get

$$\tau_u \frac{dn_+(t)}{dt} = -n_+(t) \sum_{m=0}^{\frac{M+1}{2}} s_m(t) + (1 - n_+(t)) \sum_{m=\frac{M+3}{2}}^M s_m(t). \quad (\text{S6})$$

In the  $\tau_u \rightarrow 0$  limit, Eq.S6 reduces to Eq.S5.

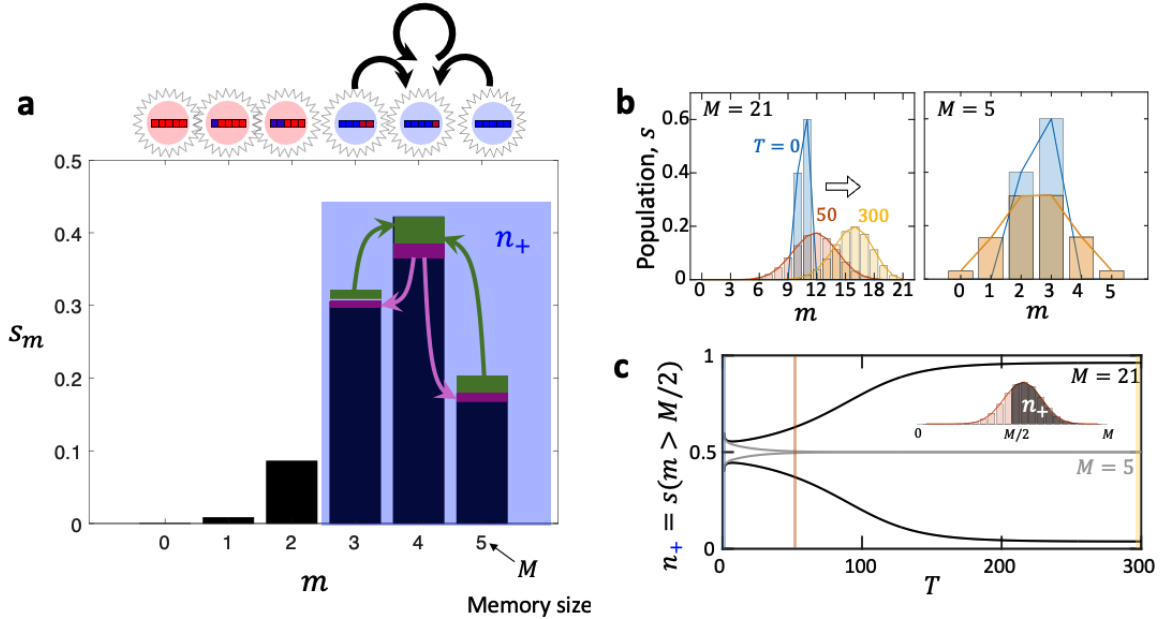

FIG. S1. **Population change over time.** **a** In a system with memory size of  $M = 5$ , the current population of agents with 4 bits of + come from previous populations with 3, 4, and 5 bits of +. **b** Population change over time for  $M = 21$  and  $M = 5$  after 50 and 300 time steps. The results are qualitatively different, with the former enhancing the initial asymmetry and the latter healing the asymmetry. **c** The total + population over time for  $M = 21$  and  $M = 5$ .

## 2. Fix points and steady states

The fixed point of the dynamics are determined by the set of equations

$$\frac{ds_m(t)}{dt} = 0 \quad \forall m \quad \text{and} \quad \frac{dn_+(t)}{dt} = 0. \quad (\text{S7})$$

The first equation implies that  $\vec{S} = (s_0, \dots, s_M)^T$  has to be in the null space of  $T$ . This shows the steady-state solution for the population with  $m$  bits of  $+$  is

$$s_m = \binom{M}{m} p_+^m p_-^{M-m}. \quad (\text{S8})$$

Being the matrix  $T$ -dependent on  $n_+$ , its null space is a function of  $n_+$ .

The fixed point of the dynamics must also satisfy  $\dot{n}_+ = 0$  in Eq.S6, implying

$$n_+ - \sum_{m=\frac{M+1}{2}}^M \binom{M}{m} p_+^m p_-^{M-m} = 0. \quad (\text{S9})$$

### 3. Effective potential landscape and quadratic approximation

If we denote the left hand side of Eq.S9 as  $V' = f(n_+)$  where the prime denotes the derivative with respect to  $n_+$ , Fig.S6 shows the  $+$  population follows differential equation  $\dot{n}_+ = -V'$  with the potential  $V$  satisfying

$$V' = n_+ - \sum_{m=\frac{M+1}{2}}^M \binom{M}{m} p_+^m p_-^{M-m}. \quad (\text{S10})$$

To show how  $M$  and  $\eta$  changes the opening direction of the potential at  $n_+ = 1/2$ , we approximate the quadratic term of the potential  $V$ . First, we evaluate the second derivative with respect to  $n_+$ .

$$V'' = \frac{\partial f}{\partial n_+} = 1 - (1 - 2\eta) \sum_{m=\frac{M+1}{2}}^M \binom{M}{m} \left( m p_+^{m-1} p_-^{M-m} - p_+^m (M - m) p_-^{M-m-1} \right). \quad (\text{S11})$$

Evaluation at  $n_+ = 1/2$  (i.e.  $p_+ = p_- = 1/2$ ) gives

$$V''|_{n_+=1/2} = 1 - (1 - 2\eta) 2^{1-M} \sum_{m=\frac{M+1}{2}}^M \binom{M}{m} (2m - M). \quad (\text{S12})$$

For large  $M$ ,  $\binom{M}{m}$  can be approximated by a normal distribution scaled in magnitude (by  $2^M$ )

$$\binom{M}{m} \approx \frac{2^M}{\sqrt{2\pi\sigma^2}} \exp\left(-\frac{(m - M/2)^2}{2\sigma^2}\right) \quad (\text{S13})$$

where  $\sigma^2 = M/4$ .

Subsequently, we approximate the sum by an integral with the aforementioned approximation of  $\binom{M}{m}$ .

$$\begin{aligned} \sum_{m=\frac{M+1}{2}}^M \binom{M}{m} (2m - M) &\approx \int_{m=M/2}^M \frac{2^M}{\sqrt{2\pi\sigma^2}} \exp\left(-\frac{(m - M/2)^2}{2\sigma^2}\right) (2m - M) dm \\ &= \frac{2^M}{\sqrt{2\pi\sigma^2}} \int_{x=0}^{M/2} \exp\left(-\frac{x^2}{2\sigma^2}\right) (2x) dx \end{aligned} \quad (\text{S14})$$

$$= \frac{2^M}{\sqrt{2\pi\sigma^2}} \int_{x^2=0}^{M^2/4} \exp(-x^2/2\sigma^2) dx^2 \quad (\text{S15})$$

$$= \frac{2^M}{\sqrt{2\pi\sigma^2}} \int_{u=0}^{M^2/8\sigma^2} \exp(-u) d(2\sigma^2 u) \quad (\text{S16})$$

$$= \frac{2^M 2\sigma^2}{\sqrt{2\pi\sigma^2}} \left[ -\exp(-u) \Big|_{u=0}^{M^2/8\sigma^2} \right] \quad (\text{S17})$$

$$= \frac{2^M \sqrt{2}\sigma}{\sqrt{\pi}} (1 - \exp(-M/2)) \quad (\text{S18})$$

$$= 2^M \sqrt{\frac{M}{2\pi}} (1 - \exp(-M/2)) \quad (\text{S19})$$

$$\approx 2^M \sqrt{\frac{M}{2\pi}}. \quad (\text{S20})$$

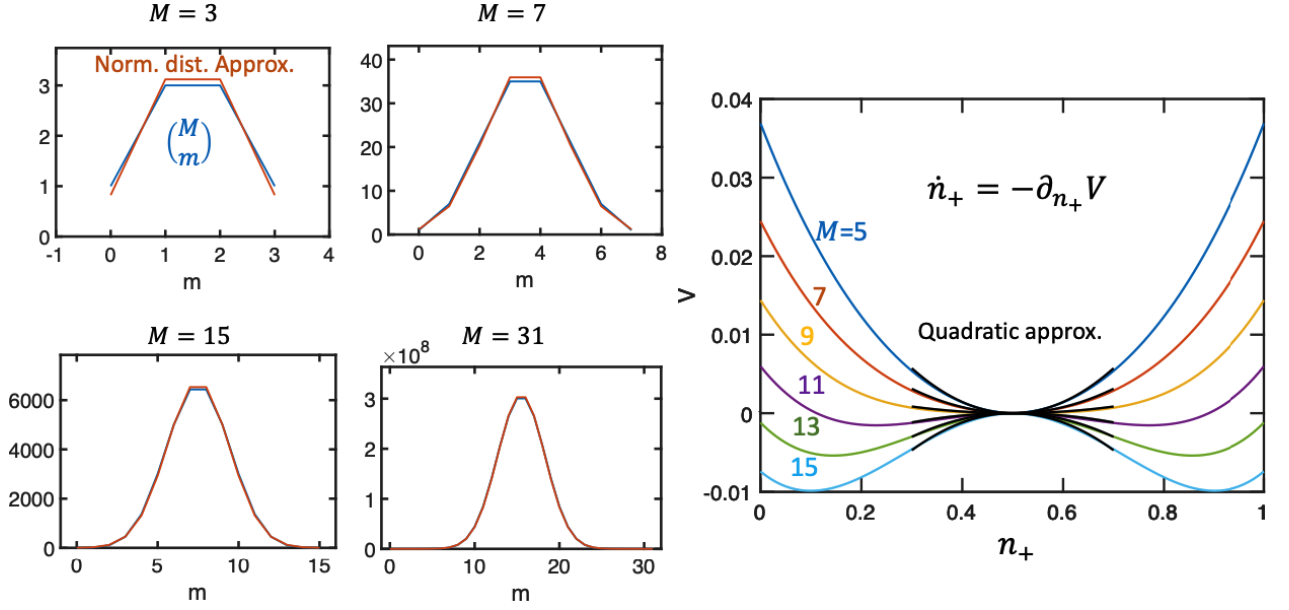

FIG. S2. **Approximations.** Left: The approximation of  $\binom{M}{m}$  by normal distribution gets closer as  $M$  increases. Right: the neighborhood around  $n_+ = 0.5$  is well approximated by the quadratic approximation (Eq.S23).

Plugging the above into Eq.S12 gives

$$V''|_{n_+=1/2} = 1 - (1 - 2\eta)2^{1-M}2^M \sqrt{\frac{M}{2\pi}} \quad (\text{S21})$$

$$= 1 - (1 - 2\eta)\sqrt{\frac{2M}{\pi}}. \quad (\text{S22})$$

indicating

$$\begin{aligned} V(n_+) &= \frac{1}{2}V''|_{n_+=1/2}(n_+ - \frac{1}{2})^2 + O(n_+^4) \\ &= \frac{1}{2} \left[ 1 - (1 - 2\eta)\sqrt{\frac{2M}{\pi}} \right] (n_+ - \frac{1}{2})^2 + O(n_+^4). \end{aligned} \quad (\text{S23})$$

The flip of the sign of the prefactor  $1 - (1 - 2\eta)\sqrt{2M/\pi}$  changes the landscape from one well to two wells. The critical memory size is therefore  $M_c = \pi/2(1 - 2\eta)^2$ . A systematic scan of the symmetry breaking characterized by the variance of the population  $\sum_i (n_{+,i} - 0.5)^2 p_i$  agrees with this criticality. The dependence on the detection error and memory size qualitatively resembles the dependence of the polarization of political agents on the tolerance to and exposure to opinions of agents which decrease opinion difference between similar agents and increase the difference otherwise (Attraction-Repulsion Model, ARM) [1]. The memory size is not the same but can be analogous to the opinion exposure at certain limit. Let us explain this in more detail. When the memory size  $M$  is relatively small compared to the total number of agents  $N$  (say, if  $N = 8$  then  $M = 1, 3, 5$  could be considered small), and the agents are dispersed across the arena, the most recent  $M$  interactions that a spinner can remember are likely to involve different agents. In this context, the memory size  $M$  effectively represents the level of opinion exposure, i.e. how many different agents across the population influence the decision-making of a single agent. On the other hand, both detection error and tolerance are measurements of the accuracy of opinion difference evaluation.

While the polarization is simultaneous in ARM so that the two extreme populations coexist, the polarization in the spinners is a spontaneous symmetry breaking. Depending on the initial condition, the agents either all become left or right and stay in that state for a very long time before some noise agitates the system to hop into the other extreme state. Nonetheless, the ensemble average of these two states resembles the polarized population in ARM.

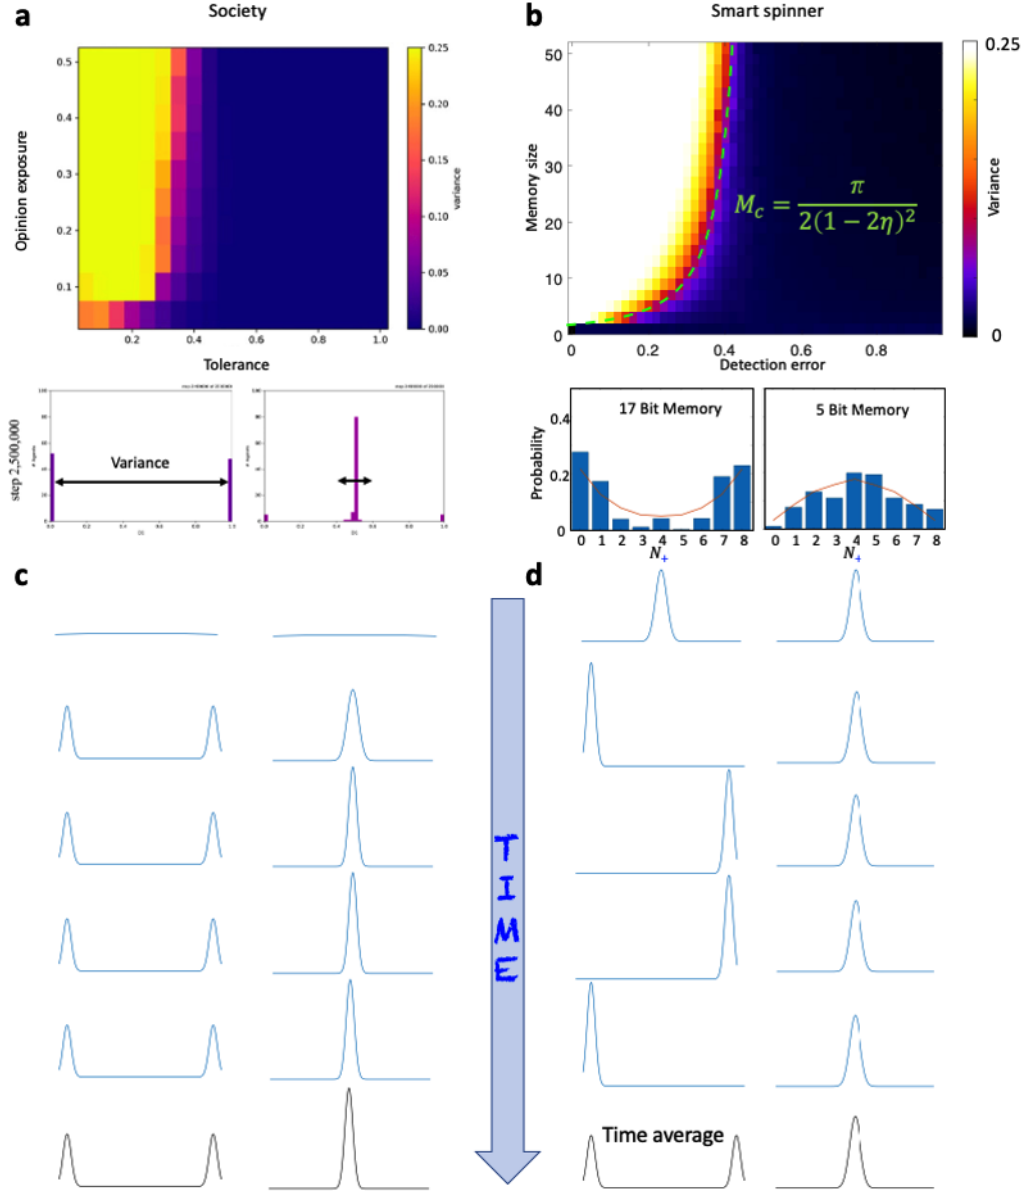

FIG. S3. **Resemblance to polarization of public opinions.** **a.** The variance of opinion from ARM. **b.** The variance of spin state from mnemonic spinners measured from state simulations (see Sec.IV B). **c.** The polarization in ARM. **d.** The polarization in the spinners.

### B. Population distribution of $N_+$ for $M = 1$ and the symmetry for transient memory

Consider  $N$  agents with transient memory, where each agent can only retain a single bit of information i.e.  $M = 1$ . Each agent remembers only the most recent interaction and makes decisions based solely on that. In other words, the agents exhibit “memoryless” behavior.

Let us look at a collision between two agents with memory states  $s_1$  and  $s_2$ , where the subscripts 1 and 2 represent which agents. After the collision, the memory states of the agents transition to  $s'_1$  and  $s'_2$  with probability  $P(s_1 s_2 \rightarrow s'_1 s'_2)$ . Since the agents are “memoryless”, all transitions are time-reversible Markovian, i.e.

$$P(s_1 s_2 \rightarrow s'_1 s'_2) = P(s'_1 s'_2 \rightarrow s_1 s_2) . \quad (\text{S24})$$

Thus, every microstate within the accessible state space has an equal likelihood, leading to equipartition of states.

The probability for the system being in a macrostate with a fraction  $n_+$  of agents in the  $+$  state, denote as  $P(n_+)$ , is therefore proportional to its multiplicity, i.e. the number of microstates corresponding to that macrostate. Thus,

$P(n_+)$  is a binomial distribution:

$$P(n_+) = \binom{N}{n_+} 2^{-N}. \quad (\text{S25})$$

In other words, when  $M = 1$ , the most likely macrostate is always at  $n_+ = 1/2$ . However, spontaneous symmetry breaking can emerge for deeper memory. We have already seen in the previous subsection that, for larger  $M$ , there can be two most likely macrostates, located at  $n_+ = 0$  and  $n_+ = 1$ .

### C. Curmudgeons bias the double-well

We can approximate the scenario with curmudgeons among pushovers by adding constant spins to the all-pushover case shown above. We consider a unity population with  $\tilde{n}_+$  share of  $+$  agents and the rest  $(1 - \tilde{n}_+)$  agents in  $-$  state. The probability to detect a  $+$  agent is now

$$p_+ = \frac{\tilde{n}_+}{1 + n_C}(1 - \eta) + \frac{1 + n_C - \tilde{n}_+}{1 + n_C}\eta \quad (\text{S26})$$

where  $n_C$  is the population ratio between the curmudgeons and the pushover. For instance, when there is 1 curmudgeon in a total of 8 agents,  $n_C = 1/(8 - 1) = 1/7$ . When  $n_C = 0$ ,  $p_+$  and  $p_-$  reduce to Eq.S2.

By plugging  $p_+$  of Eq.S26 into Eq.S10, we get  $V(\tilde{n}_+)$  for a system with curmudgeons and pushovers. The rescaled  $+$  population considering the constant curmudgeons is  $n_+ = (\tilde{n}_+ + n_C)/(1 + n_C)$ . The plot showing the  $V$  in terms of  $n_+$  for different amount of curmudgeon (constant agents) is shown in Fig.S5.

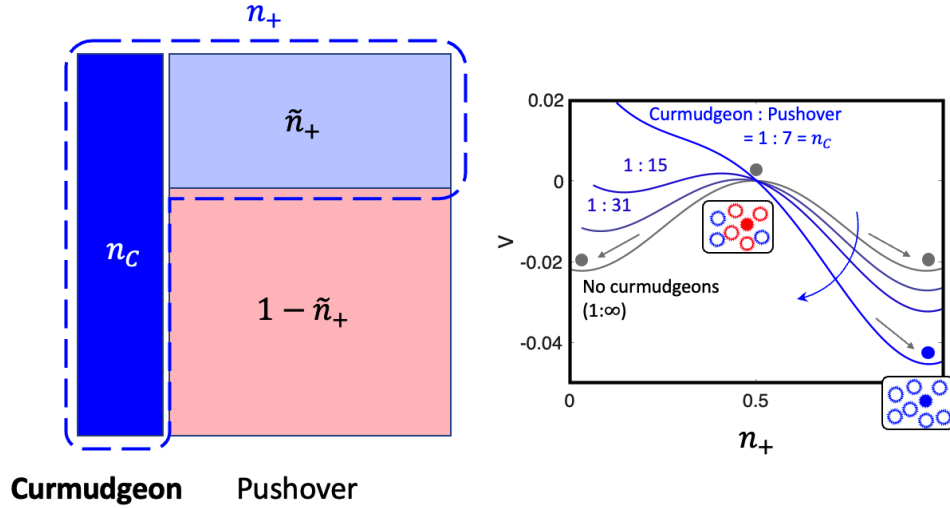

FIG. S4. **Constant curmudgeons bias the symmetric double well.** **a** The curmudgeon can be regarded as a constant population with  $+$  spin in addition to the flow-able population of  $+$  and  $-$  pushovers. **b** Higher Curmudgeon-to-Pushover ratio ( $n_C$ ) biases the double well more.

### D. A contrarian oscillates the demographics

The normalized population of pushovers in the  $+$  state excessive over  $1/2$ ,  $p = n_+ - 1/2$ , affects and is affected by the normalized  $+$  bits excessive over  $1/2$  in the contrarian  $c = m_C/M - 1/2$ .  $c$  determines the state of the contrarian such that the contrarian is in the  $+$  state and  $-$  state when  $c > 0$  and  $c < 0$ , respectively, such that

$$dc/dt = k_c p + \xi_c. \quad (\text{S27})$$

The state of the contrarian sets the landscapes such that

$$dp/dt = -k_p \text{sgn} c + \xi_p. \quad (\text{S28})$$

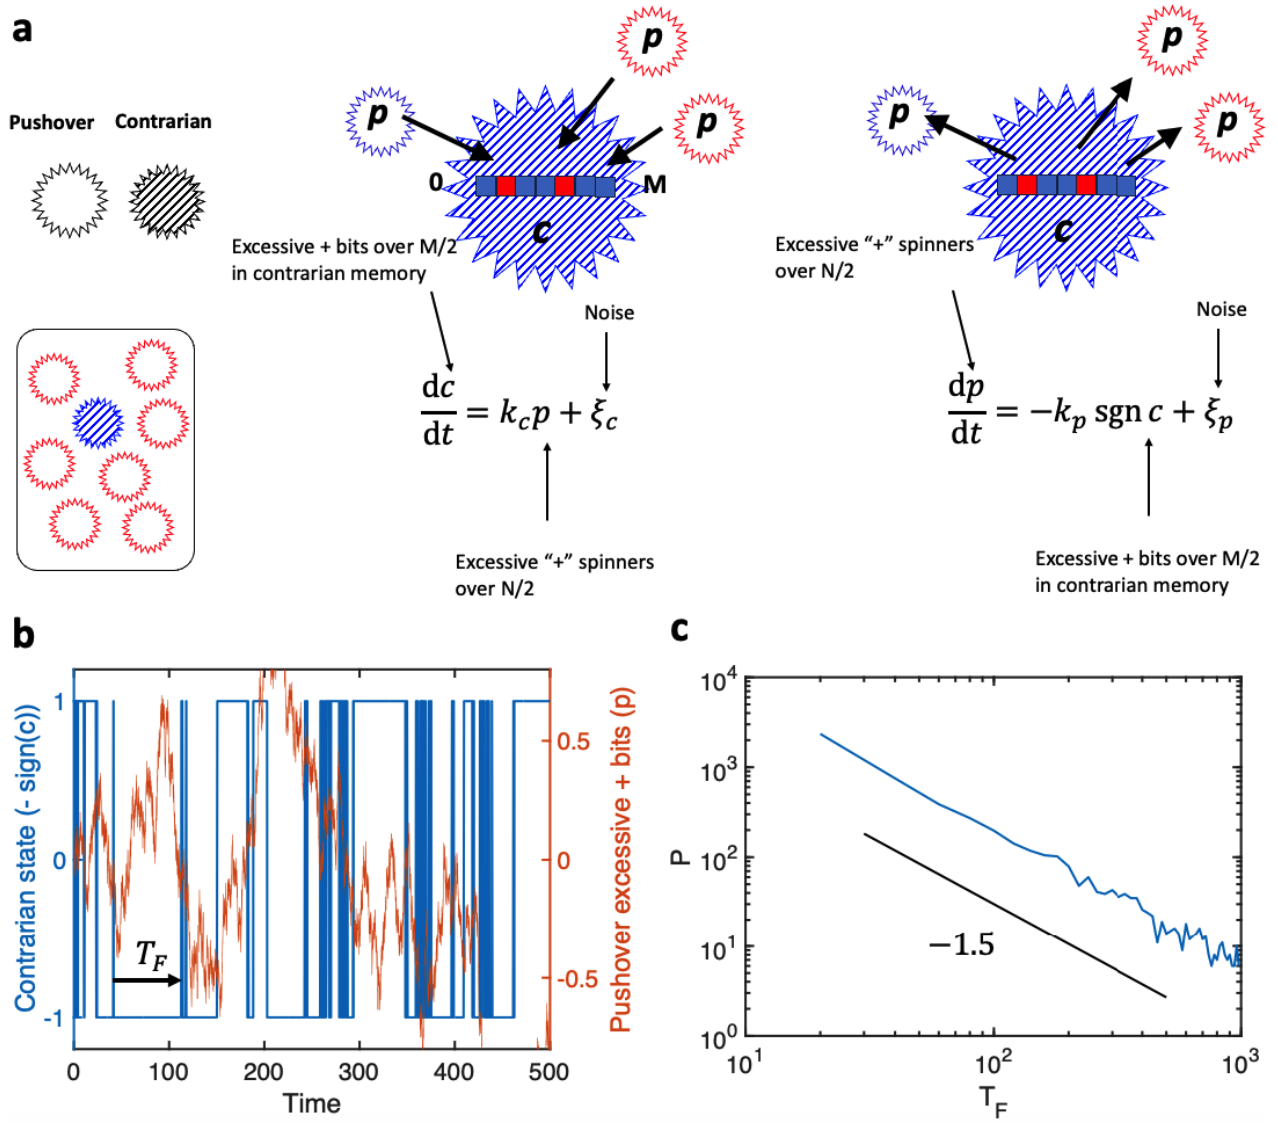

FIG. S5. **Contrarian-pushover model.** **a** The pushovers keep notifying the contrarian the current demographics. The contrarian impose an opposite drive to change the demographics of pushovers. **b** Contrarian state and pushover population over time by integrating Eq.S27 and Eq.S28 using  $k_p = k_c = 0.01$ ,  $\xi_p, \xi_c \sim U[-10, 10]$ , and  $dt = 0.001$ . **c** The statistics of flipping time  $T_F$  shown in **b** and a comparison with a power law with exponent  $-1.5$ .

## II. SUPPLEMENTARY EXPERIMENT TRAJECTORIES

Figures S6 - S9 show the raw data supporting the main text.

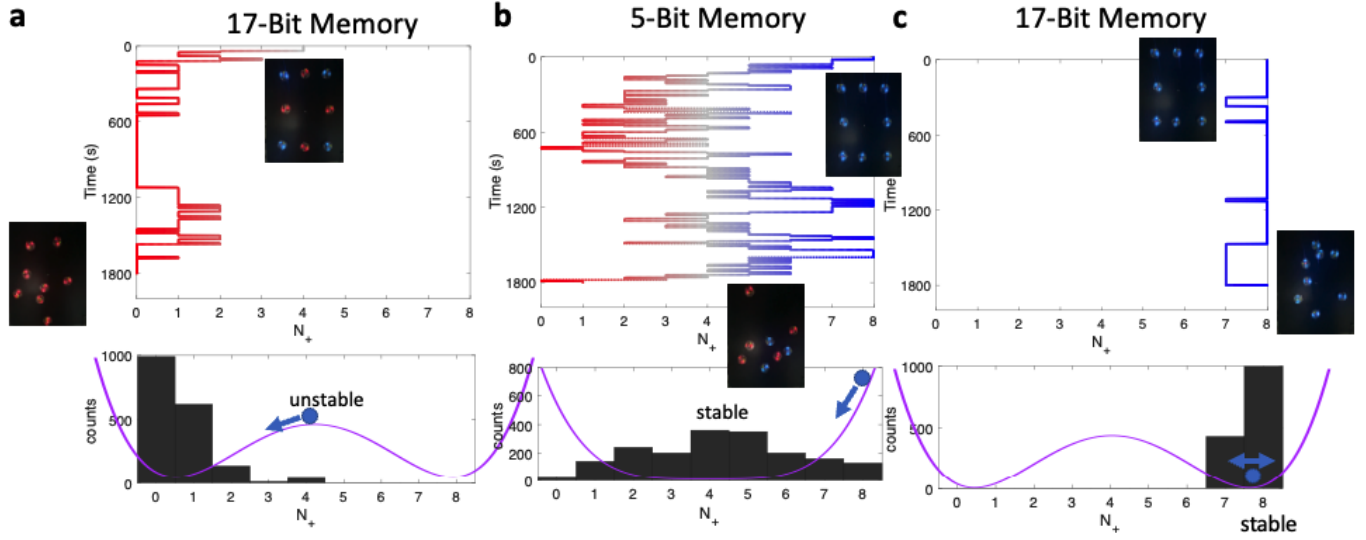

FIG. S6. **All-pushover experiments with different memory depths.** **a.** Agents with 17-bit memories create a landscape unstable at 50/50 that a system started at 50/50 falls into a red-dominant state. **b.** Agents with 5-bit memories create a landscape stable at 50/50 and shows higher probabilities closer to 50/50. **c.** When agents with 17-bit memories directly start at the other valley of the double-well landscape, the blue-dominant valley, the system stays in the state.

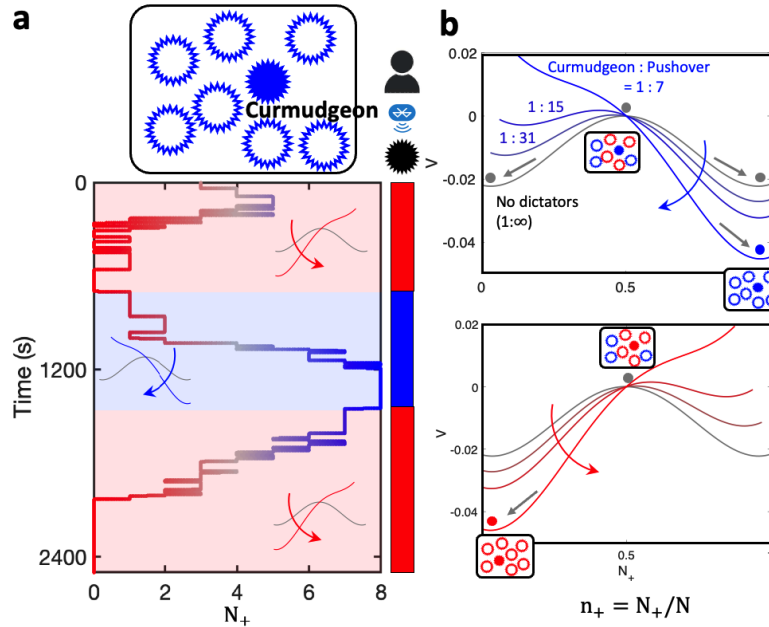

FIG. S7. **A remote-controlled curmudgeon.** **a.** One agent (curmudgeon) is controlled by using Low Energy Bluetooth (BLE) among the other seven pushovers with  $M = 17$ . As this agent is switched to blue (+), the landscape of biases to be blue-dominant. Similarly, the landscape biases to red when the curmudgeon is switched by the remote control to red (-). In the experiment, we first let the curmudgeon be constantly red. The pushovers gradually become red-dominant as following the red-biased landscape. After all agents became red, we remotely switched the curmudgeon to blue. The pushovers are brought to the blue-dominant state again. Finally, we switched the curmudgeon to red and the pushovers are converted to red-dominant state. From this we can see the pushover can always follow the curmudgeon given the condition for biased double-well is met. **b** How the symmetric double well is deformed to biased double wells.

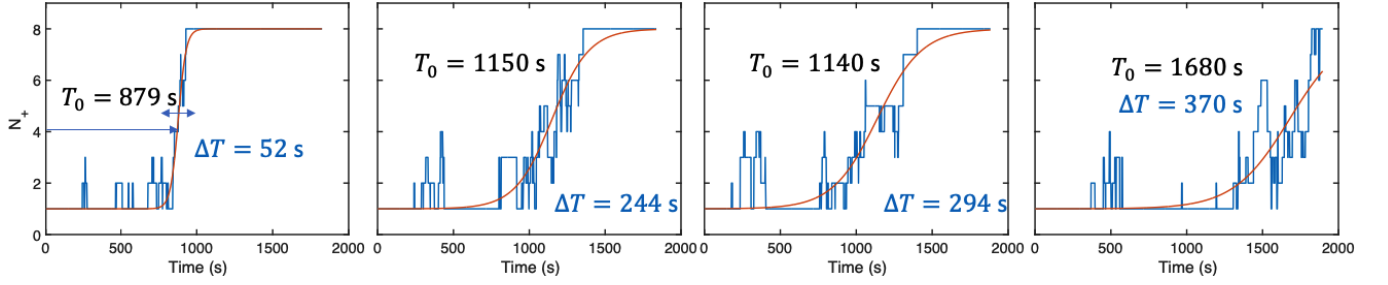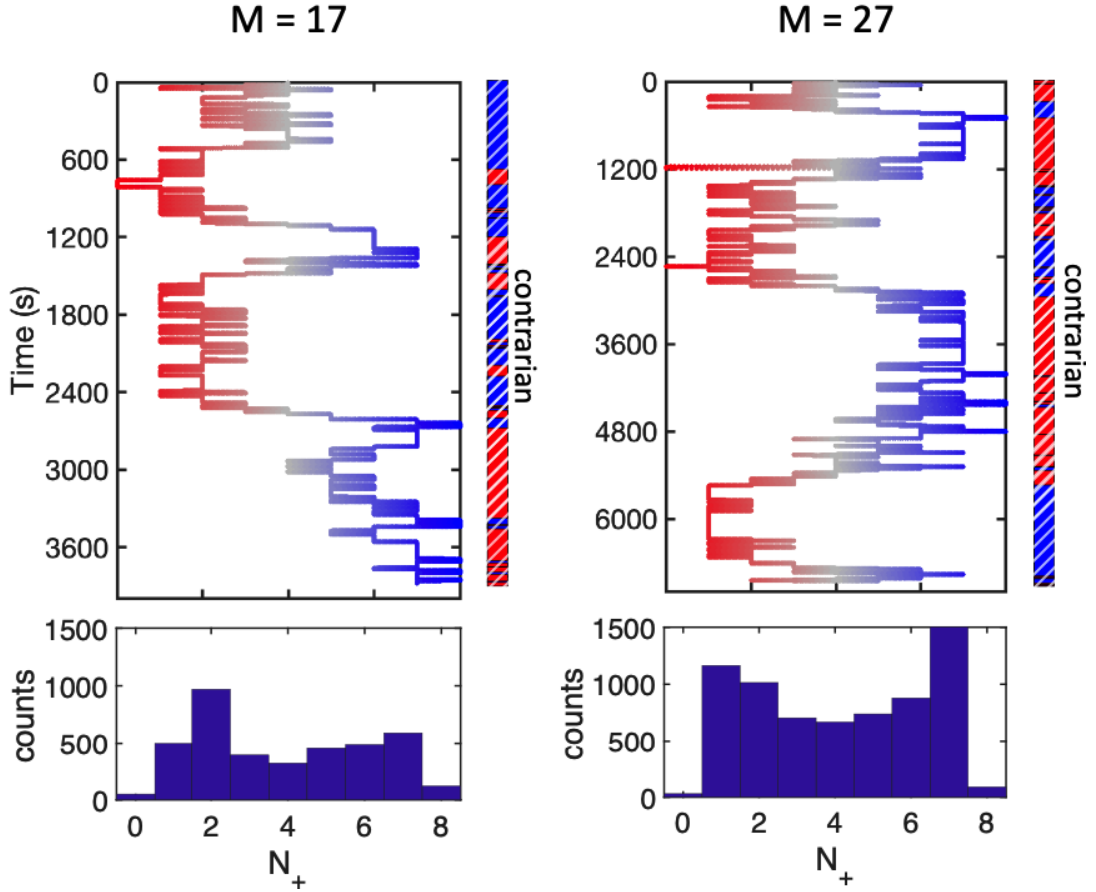

### III. ALGORITHMS FOR ROBOTIC AGENTS

In addition to the algorithm for pushovers, here is the algorithm for the contrarian and time-weighted agents (traditionalist, pushover, opportunist). The only change for the pseudo algorithm is the weighting part, which is shown in red.

---

**Algorithm S1** Detection and actuation with weights

---

```

1:  $z$  = current angular velocity
2:  $std0$  = the variance of acceleration in the past 0.1 s
3: if  $std0 > s0$  then
4:    $r = (\omega_{old} - z) / \omega_{old}$ 
5:   if  $|\omega_{old}| > 30$  (deg/s) then
6:     if  $\omega_{old} > 0$  then
7:       if  $r < 0.3$  then
8:         Push  $-1$  into the memory
9:       else
10:        Push  $+1$  into the memory
11:      end if
12:    end if
13:    if  $\omega_{old} < 0$  then
14:      if  $r < 0.3$  then
15:        Push  $+1$  into the memory
16:      else
17:        Push  $-1$  into the memory
18:      end if
19:    end if
20:  end if
21:   $ccw = \sum_{i=1}^M w_i \cdot \mathbb{1}[q_i = +1]$  where  $q_i$  is the latest bit.
22:   $cw = \sum_{i=1}^M w_i \cdot \mathbb{1}[q_i = -1]$  where  $q_i$  is the latest bit.
23:  if  $ccw > cw$  then
24:     $s_{other} = 1$ 
25:  end if
26:  if  $s_{other} \cdot s < 0$  then
27:     $s = -s$ 
28:  end if
29: end if
30:  $\omega_{old} = z$ 

```

---

## IV. SIMULATION

### A. Molecular dynamics simulation

The mechanical model of the spinners and the physical parameters (mass, size, measured translational and rotational damping and drive, air current force are the same as described in SI document of [2].

In addition to the mechanical model, the response and actuation of the microcontroller follow exactly the same as the Arduino codes (using algorithms 1 and S1) uploaded to the spinners. The detection error from this simulation reproduces observations in experiments, which is about 30%.

|                  | Description                             | Value                                  | Reference                                       |
|------------------|-----------------------------------------|----------------------------------------|-------------------------------------------------|
| $m$              | Spinner mass                            | 0.053 kg                               | Direct measurement from a scale                 |
| $R_0$            | Spinner outer radius                    | 0.038 m                                | Direct measurement from a caliper               |
| $R_i$            | Spinner inner radius                    | 0.030 m                                | Same as above                                   |
| $I$              | Spinner moment of inertia               | $2.5 \times 10^{-5} \text{ kg m}^2$    | $\approx 0.33 m R_0^2$                          |
| $\Omega$         | Saturated angular velocity of the orbit | 28 rad s <sup>-1</sup>                 | Measurement from experiment videos              |
| $\gamma$         | Rotational driving acceleration         | 1.5 rad s <sup>-2</sup>                | Same as above                                   |
| $\tau_{drive}^0$ | Rotational driving torque               | $3.8 \times 10^{-5} \text{ N m}$       | $= I\gamma$                                     |
| $\eta$           | Translational drag coefficient          | $3.4 \times 10^{-3} \text{ kg s}^{-1}$ | $= m \cdot 6.5 \times 10^{-2} \text{ s}^{-1}$ . |
| $\eta_\varphi$   | Rotational drag coefficient             | $1.34 \times 10^{-6} \text{ N m s}$    | $= \tau_{drive}/\Omega$                         |
| $F_{air}$        | Air current force                       |                                        | See [2].                                        |
| $A_1$            | Half arena length                       | 0.38 m                                 | Direct measurement from a meter stick           |
| $A_2$            | Half arena width                        | 0.28 m                                 | Same as above                                   |

TABLE S1. List of parameters used in the Molecular-Dynamics-type simulations.

### B. Simplified state simulation

We simplify that the agents are not moving but reading the other spinners with a fix error rate (30%) while in the actual experiments, the error rate is fluctuating about that mean.

## V. SUPPLEMENTARY MOVIES

### [SI1] Smart spinner introduction

The movie includes: 1. the actuation of counterclockwise and clockwise spins, 2. the mechanisms of opposite-spin and opposite-spin interactions, 3. how the mechanism in 2. helps the spinners with sensors detect the spin of another spinner, 4. how a spinner copies the sign of another spinner based on 3., 5. how the readings of other spinners are pushed into a spinner with memory from other constant spinners (+ in this particular video) and make the spinner with memory change its state.

### [SI2] Spontaneous symmetry breaking of the pushovers

The movie shows the statistics of the states over time for  $M = 1$  and  $M = 17$ . Spontaneous symmetry breaking can be seen in the  $M = 17$  case but not in the  $M = 1$  case.

### [SI3] Curmudgeon leading the pushovers

The movie shows how the double-well landscape at  $M=27$  is biased with the introduction of curmudgeons. The movie displays the landscape shape for curmudgeon:pushover = 0:32, 1:31, 1:15, and 1:7. Then, the movie displays an experiment video with one curmudgeon and seven pushovers with  $M=27$ . Finally, a bluetooth-controlled curmudgeon directs the population at the will of the lab member controlling the remote control.

### [SI4] Contrarian oscillates the climate

This movie shows an experiment with one contrarian and seven pushovers with  $M=17$ . The number of + agents that change over time in the landscape changing in conjunction with the contrarian state is displayed in sync with the video of the experiment.

### [SI5] Traditionalists and opportunists

The movie shows the experiments of 8 traditionalists ( $b = 0.5$ ), 8 pushovers ( $b = 1$ ), and 8 opportunists ( $b = 2$ ), respectively, with temporal weights for memory  $w(t) = b^t$ . The agents all start with  $-$  state with all bits being  $-$  in memory. The memory sizes all use  $M = 9$ . It can be observed that the opportunists melt to 50/50 the fastest, followed by the traditionalists, with the pushovers being significantly slower due to the proximity to the critical memory size.

### [SI6] Simulations

The movie first shows the simulation close-ups of a same-spin collision and opposite-spin collision. Then it displays the mechanical inference of the spins. The inference result of the spinner in contact is shown as solid dots in the center. The correctness of the inference is annotated with text. The statistics on the side of the movie shows a detection correctness of 70%, matching experiment measurements. Finally, the movie shows the simulations of a curmudgeon-pushover system, a contrarian-pushover system, and a weighted-memory system corresponding to the experiment videos in SI3.mp4, SI4.mp4, and SI5.mp4.

- 
- [1] R. Axelrod, J. J. Daymude, and S. Forrest, Proceedings of the National Academy of Sciences **118**, e2102139118 (2021).
  - [2] S. Li, T. V. Phan, G. Wang, R. Khuri, J. W. Wilson, R. H. Austin, and L. Liu, Communications Physics **7**, 136 (2024).
